# Supplementary material for: Pregeometric Origins of Liquidity Geometry in Financial Order Books
Source: arXiv:2601.17245 source file (2026-01-24)
Supplement: Supplementary file 1 [file Supplementary.pdf]

# Supplementary Material for
# *Pregeometric Origins of Liquidity Geometry in Financial Order Books*

João P. da Cruz
(Dated: January 23, 2026)

## S1. MODEL COMPARISON METHODOLOGY

This Supplementary Material is intended to provide robustness checks and diagnostics supporting the main empirical claims, not to introduce additional model assumptions.

This Supplementary Material provides additional validation of the empirical results presented in Sec. **??** of the main text. In particular, we report explicit model comparison and residual diagnostics designed to assess whether the integrated-gamma geometry provides a genuinely superior description of cumulative order-book liquidity.

### A. Competing cumulative models

For each asset, book side, and intraday window, the empirical cumulative liquidity profiles $\overline{S}(x)$ are fitted using the following competing models:

1. **Integrated-gamma model** (main text):

$$S_\Gamma(x) = \frac{C}{\lambda^{\gamma+1}}\,\gamma(\gamma+1, \lambda x),$$

   with three free parameters $(C, \gamma, \lambda)$.

2. **Log-normal cumulative model**:

$$S_{\rm LN}(x) = A\,\Phi\!\left(\frac{\log x - \mu}{\sigma}\right),$$

   where $\Phi$ denotes the standard normal cumulative distribution function and $(A, \mu, \sigma)$ are free parameters.

3. **Truncated power-law cumulative model**:

$$S_{\rm PL}(x) = B\,x^{\alpha}, \qquad x \le x_{\rm max},$$

   with parameters $(B, \alpha)$ and an effective cutoff imposed by the fitting window.

All models are fitted over identical ranges $x = 1, \ldots, K$, with $K = 50$ unless otherwise stated. Fits are performed independently for bid and ask sides.

### B. Likelihood and information criteria

Because the observables are cumulative quantities, residuals at different $x$ are not statistically independent. We therefore adopt a pragmatic likelihood approximation based on window-wise Gaussian errors in log-space,

$$\varepsilon_{\log}(x) = \log \overline{S}_{\rm emp}(x) - \log \overline{S}_{\rm fit}(x),$$

with an effective log-likelihood

$$\log \mathcal{L} = -\frac{1}{2}\sum_x \frac{\varepsilon_{\log}(x)^2}{\sigma_{\log}^2},$$

where $\sigma_{\log}$ is estimated empirically within each window.

While this likelihood does not model the full covariance structure of cumulative data, the use of identical approximations across all competing models ensures that AIC differences reflect genuine relative model performance rather

than artifacts of the likelihood specification. We verified that rankings remain unchanged under alternative error models (linear-scale residuals, weighted least squares).

Model preference is quantified using the Akaike Information Criterion (AIC),

$$\mathrm{AIC} = 2k - 2\log\mathcal{L},$$

where $k$ is the number of free parameters. Differences

$$\Delta\mathrm{AIC} = \mathrm{AIC}_{\mathrm{alt}} - \mathrm{AIC}_{\Gamma}$$

are reported throughout; negative values indicate preference for the integrated-gamma geometry.

## S2. RESIDUAL DIAGNOSTICS

To assess whether deviations from the integrated-gamma form exhibit systematic structure, we perform a detailed residual analysis.

### A. Residuals versus distance from the mid

For each asset, side, and intraday window, we compute log-residuals $\varepsilon_{\log}(x)$ as defined above. Figure 1(a) shows the median and interquartile range of $\varepsilon_{\log}(x)$ as a function of tick distance from the mid.

Across all assets, residuals collapse tightly around zero beyond the first few ticks. Systematic deviations are confined to the innermost levels ($x \lesssim 3$), where discrete price grids, queueing effects, and matching rules dominate and where the continuum projection underlying the model is not expected to apply.

### B. Residual distributions

Figure 1(b) reports the pooled distribution of log-residuals across assets, sides, and intraday windows. The distribution is sharply peaked at zero and approximately symmetric, with rapidly decaying tails. No evidence of heavy-tailed or skewed residual structure is observed.

### C. Autocorrelation of residuals

Figure 1(c) shows the autocorrelation function of log-residuals across tick distance. Correlations decay rapidly and vanish beyond the first few bins, indicating the absence of long-range structure not captured by the integrated-gamma geometry. The short-range correlations observed at the smallest lags are consistent with tick discretization effects rather than with a failure of the assumed functional form.

## S3. REPRODUCIBILITY AND SCOPE

All empirical results are obtained using identical preprocessing, binning, and fitting procedures across assets. Parameter estimation and model comparison are performed independently for each intraday window, ensuring that reported statistics are not dominated by outliers or specific market conditions.

The analysis is intentionally local in time and restricted to a finite window around the mid price. No claims are made regarding behavior at extreme distances or during auction phases. Within this scope, the integrated-gamma geometry provides a parsimonious and structurally validated description of projected liquidity.

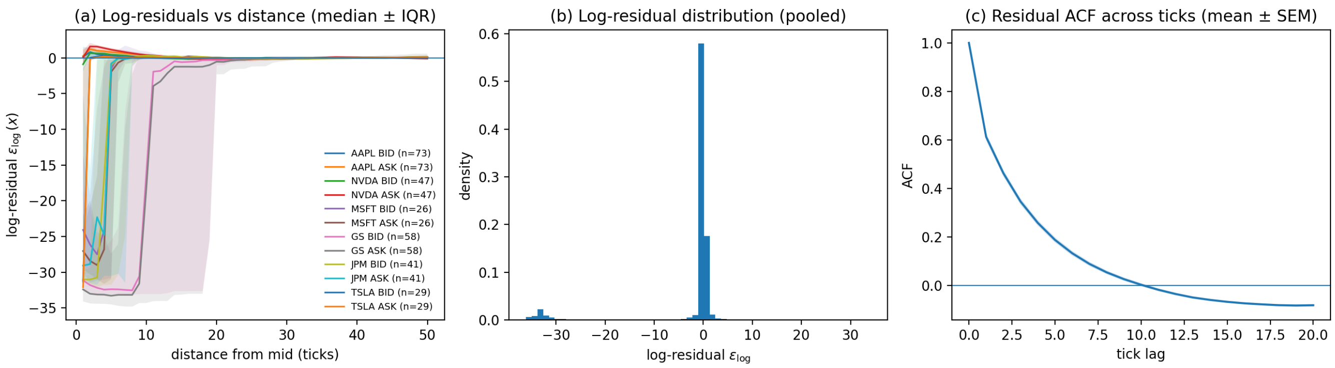


FIG. 1: **Residual diagnostics for integrated-gamma liquidity geometry.** (a) Median log-residuals and interquartile ranges as a function of distance from the mid price, shown separately for each asset and side. Residuals collapse around zero beyond the innermost ticks. (b) Pooled distribution of log-residuals across all assets, sides, and windows. (c) Autocorrelation function of log-residuals across tick distance, averaged over windows; correlations decay rapidly, indicating absence of long-range structure beyond tick-scale discretization effects.
